# Supplementary material for: ANLIzing the Adversarial Natural Language Inference Dataset
Source: arXiv:2010.12729 source file (2020-10-24)
Supplement: Supplementary file 1 [file appendix_incidence_counts_by_label.tex]

\begin{table*}[t]
    \centering
    \small
\begin{tabular}{ccrrrrrr}
\toprule
\bf Dataset & \bf Gold Label & Numerical &  Cardinal &  Ordinal &  Counting &  Dates &  Age \\
\midrule
\multirow{3}{*}{\bf A1} 
& C  &        103 &   \bf     90 &       14 &         3 &  \bf   70 &   10 \\
& N   &         29 &        27 &        2 &         0 &     22 &    0 \\
& E   &         64 &        55 &        8 &         4 &     42 &   11 \\
\midrule
 \multirow{3}{*}{\bf A2} 
& C   &         67 &        56 &       14 &         2 &     47 &    7 \\
& N   &         22 &        17 &        5 &         2 &     11 &    0 \\
& E   &         70 &        58 &        8 &         6 &     45 &    5 \\
\midrule
\multirow{3}{*}{\bf A3} 
& C   &         20 &        16 &        2 &         5 &      5 &    2 \\
& N   &          9 &         7 &        0 &         2 &      0 &    2 \\
& E   &         20 &        12 &        3 &         5 &      4 &    1 \\
 \bottomrule
\end{tabular}
    \caption{Counts of `Numerical' tag types by gold label and subdataset.
    }
    \label{tab:goldnumerical}
\end{table*}

\begin{table*}[t]
    \centering
    \small
\begin{tabular}{ccrrrrrrrr}
\toprule
\bf Dataset & \bf Gold Label  &  Basic &  Lexical &  Comp.Super. &  Modus &  CauseEff. &  Idiom &  Negation &  Conjunction \\
\midrule
 \multirow{3}{*}{\bf A1} 
& C   &     25 &       26 &                       9 &            0 &            1 &      0 &         4 &            6 \\
& N   &     26 &       14 &                       8 &            0 &            1 &      0 &         4 &            8 \\
& E   &     44 &       25 &                       9 &            4 &            2 &      1 &        13 &            7 \\
\midrule
 \multirow{3}{*}{\bf A2} 
& C   &     33 &       29 &                      13 &            1 &            1 &      0 &        13 &            4 \\
& N   &     26 &       20 &                      14 &            0 &            1 &      1 &         8 &            3 \\
& E   &     47 &       53 &                      17 &            2 &            3 &      0 &        15 &            5 \\
\midrule
 \multirow{3}{*}{\bf A3} 
& C   &     38 &       44 &                       6 &            1 &            6 &      4 &        14 &            8 \\
& N   &     34 &       24 &                       9 &            0 &            2 &      2 &        15 &            4 \\
& E   &     63 &       64 &                       6 &            5 &           12 &      4 &     \bf   28 &            4 \\
\bottomrule
\end{tabular}
    \caption{Counts of `Basic' tag types by gold label and subdataset.
    }
    \label{tab:goldbasic}
\end{table*}

\begin{table*}[t]
    \centering
    \small
\begin{tabular}{ccrrrr}
\toprule
\bf Dataset & \bf Gold Label  &  Ref. &  Coref. &  Names &  Family \\
\midrule
 \multirow{3}{*}{\bf A1} 
& C   &         21 &           18 &      5 &       0 \\
& N     &         16 &           16 &      0 &       0 \\
& E   &         29 &           24 &      7 &       2 \\
\midrule
 \multirow{3}{*}{\bf A2} 
& C   &         33 &           31 &      6 &       2 \\
& N     &         38 &           33 &      3 &       3 \\
& E   &         29 &           26 &      4 &       1 \\
\midrule
 \multirow{3}{*}{\bf A3} 
& C   &         27 &           26 &      2 &       1 \\
& N     &         27 &           23 &      3 &       1 \\
& E   &         37 &           31 &      5 &       5 \\
\bottomrule
\end{tabular}
    \caption{Counts of `Reference' tag types by gold label and subdataset.
    }
    \label{tab:goldreference}
\end{table*}

\begin{table*}[t]
    \centering
    \small
\begin{tabular}{ccrrrrr}
\toprule
\bf Dataset & \bf Gold Label &  Tricky &  Syntactic &  Presupposition &  Exhaustification &  Wordplay \\
\midrule
 \multirow{3}{*}{\bf A1} 
& C   &      64 &    \bf     43 &               2 &                12 &         7 \\
& N   &      18 &          9 &               1 &                 5 &         2 \\
& E   &      35 &         12 &              15 &                 7 &         2 \\
\midrule
 \multirow{3}{*}{\bf A2} 
& C   &      49 &         18 &               3 &                17 &        11 \\
& N   &      22 &          4 &               1 &                15 &         1 \\
& E   &      33 &         10 &               5 &                10 &         7 \\
\midrule
 \multirow{3}{*}{\bf A3} 
& C   &      52 &         16 &              10 &                14 &        15 \\
& N   &      28 &          9 &               7 &                 4 &         4 \\
& E   &      55 &         16 &       \bf       25 &                 8 &        11 \\
\bottomrule
\end{tabular}
    \caption{Counts of `Tricky' tag types by gold label and subdataset.
    }
    \label{tab:goldtricky}
\end{table*}

\begin{table*}[t]
    \centering
    \small
\begin{tabular}{ccrrrrrr}
\toprule
\bf Dataset & \bf Gold Label  &  Reasoning &  Likely &  Unlikely &  Debatable &  Facts &  Containment \\
\midrule
 \multirow{3}{*}{\bf A1} 
& C   &         62 &       5 &         2 &          3 &     44 &           11 \\
& N   &   \bf     151 &  \bf   113 &        27 &          3 &      6 &            6 \\
& E   &         56 &       4 &         1 &          8 &     29 &           21 \\
\midrule
 \multirow{3}{*}{\bf A2} 
& C   &         71 &       2 &         7 &          7 &     56 &           17 \\
& N   &    \bf    141 &  \bf   113 &        19 &         14 &      8 &            5 \\
& E   &         86 &       2 &         0 &         16 &     58 &           15 \\
\midrule
 \multirow{3}{*}{\bf A3}
& C   &         65 &       7 &         4 &         14 &     45 &            5 \\
& N   &   \bf     168 &      93 &        33 &     \bf    47 &   \bf  23 &            6 \\
& E   &         84 &   \bf   24 &         1 &         13 &     53 &            9 \\
\bottomrule
\end{tabular}
    \caption{Counts of `Reasoning' tag types by gold label and subdataset.
    }
    \label{tab:goldreasoning}
\end{table*}

\begin{table*}[t]
    \centering
    \small
\begin{tabular}{ccrrrrrr}
\toprule
\bf Dataset & \bf Gold Label &  Imperfections &  Label &  Ambiguity &  EventCoref &  Translation &  Spelling \\
\midrule
\multirow{3}{*}{\bf A1} 
& C   &       16 &      6 &          2 &           1 &            2 &         7 \\
& N   &       14 &      6 &          0 &           0 &            0 &         7 \\
& E   &       19 &      9 &          1 &           0 &            2 &         4 \\
\midrule
 \multirow{3}{*}{\bf A2} 
& C   &       12 &      3 &          2 &           5 &            3 &         7 \\
& N   &       18 &      6 &          0 &           8 &            1 &        10 \\
& E   &       15 &      6 &          2 &           0 &            1 &         7 \\
\midrule
 \multirow{3}{*}{\bf A3} 
& C   &       23 &      2 &    \bf     11 &           9 &            0 &         2 \\
& N   &     \bf  37 &      8 &    \bf     16 &           8 &            2 &         9 \\
& E   &       22 &      5 &     \bf    12 &           0 &            0 &         8 \\
\bottomrule
\end{tabular}
    \caption{Counts of `Imperfections' tag types by gold label and subdataset.
    }
    \label{tab:goldquality}
\end{table*}
