# Supplementary material for: ANLIzing the Adversarial Natural Language Inference Dataset
Source: arXiv:2010.12729 source file (2020-10-24)
Supplement: Supplementary file 4 [file appendix_transformer_acc_table.tex]

\begin{table}[t]
    \centering
    \small
    \begin{adjustbox}{max width=\linewidth}
    \begin{tabular}{lcc}
    \toprule
    \bf Model & Data & Acc.$_{M/MM}$ \\
    \midrule
    BERT (R1)$^*$ & S+M & 0.867 / 0.864 \\
    RoBERTa Ens. (R2)$^*$ & S+M+F+A1 & 0.909 / 0.907  \\
    RoBERTa Ens. (R3)$^*$ & S+M+F+A12 & 0.910 / 0.907  \\\midrule
    BERT-base-uncased & S+M+F+A123 & 0.852 / 0.851  \\
    distilBERT-base &  S+M+F+A123 & 0.823 / 0.830  \\
    RoBERTa-base &  S+M+F+A123 & 0.876 / 0.874  \\
    distilRoBERTa-base &  S+M+F+A123 & 0.841 / 0.843  \\
    AlBERT-base &  S+M+F+A123 & 0.854 / 0.853 \\
    XLNet-base &  S+M+F+A123 & 0.870 / 0.868  \\
    \bottomrule
    \end{tabular}
    \end{adjustbox}
    \caption{Training data and development set accuracies (`M.' refers to MultiNLI matched dev., `MM' refers to MultiNLI 
    mismatched dev.) for all 9 compared models. $^*$ denotes that the model in question was used to collect one of the rounds of ANLI, and their numbers are reported, `Ens.' refers to an ensemble.
    }
    \label{tab:models}
\end{table}
